# Supplementary material for: Quantum gravitational corrections to Reissner-Nordstr\"om black hole thermodynamics and their implications for the weak gravity conjecture
Source: arXiv:2503.08459 ancillary file (2026-07-03)
Supplement: Supplementary file 1 [file attached_Notebook_for_WGC_v3.pdf]

Note : The file uses the package "diffgeoM.m", which can be downloaded from : <https://github.com/bryango/diffgeoM>.

## \* Verification of the weak gravity conjecture by considering corrections to the charged BH thermodynamics

### 0. The original unperturbed BH solution and thermodynamics:

We should be familiar with the properties of original unperturbed BH, which includes the gravitational and the electromagnetic sectors.

```
In[1]:= coord = {t, r,  $\theta$ ,  $\phi$ };  
$Assumptions =  
默认假设  
And[t  $\in$  Reals, M  $\in$  Reals, r  $\in$  Reals, r > 0,  $0 < \phi < 2\pi$ ,  $0 < \theta < \pi$ , M > 0];  
逻辑与 实数域 实数域 实数域  
metricsign = -1;  
metric = DiagonalMatrix[{- (f[r]), 1 / (f[r]), r^2, r^2 * (Sin[ $\theta$ ]) ^2}];  
对角矩阵 正弦  
<< "D:\\diffgeoM.wl"  
偏导  
rie0 = lower[Riemann, {4}];
```

```
In[7]:= ff[r_] = 1 -  $\frac{2M}{r} + \frac{q^2}{r^2}$ ;  
au = {-q / r, 0, 0, 0};  
fuv = covariant[au] - Transpose[covariant[au], {2, 1}] // Simplify;  
转置 化简  
fuvup = raise[%, {1, 2}] // Simplify;  
化简  
sr[var_] := Normal[Series[var, { $\epsilon$ , 0, 1}]];  
转换... 级数  
sr0[var_] := Normal[Series[var, { $\epsilon$ , 0, 0}]];  
转换... 级数
```

( ff[r] is the concrete expression of f[r]. We make the substitution  $f \rightarrow ff$  when it is needed. )

In[13]:=

```

mh0 =  $\frac{q^2 + rh0^2}{2 rh0}$ ;
tem =  $-\frac{q^2}{4 \pi rh0^3} + \frac{1}{4 \pi rh0}$ ;
entr0 = Pi rh0^2;
      圆周率
phi0 = q / rh0;
freeqt0 = mh0 - tem * entr0 // Simplify
      化简

```

Out[17]=

$$\frac{3 q^2 + rh0^2}{4 rh0}$$

Above, we use the symbol rh0 to represent the barred quantity  $\bar{r}_h$  in our paper, which is the horizon radius of the original unperturbed black hole with the parameter T and q. Here the free energy F(T,q) is that for the thermodynamic ensemble depending on T and q.

### 1. The perturbed free energy at first order in $\epsilon$ :

According to the simple approach, at first order in  $\epsilon$ , the free energy coming from the part  $\int R - \frac{1}{4} F^2$  is given by the known form (copied from above):

In[18]:=

freeqt0

Out[18]=

$$\frac{3 q^2 + rh0^2}{4 rh0}$$

The partition function LnZ (related to Euclidean integral) coming from the higher derivative part  $\epsilon \int L_{hd}$  can be calculated by inserting the unperturbed RN solution into it.

```

In[19]:= rHd1 = RicciScalar^2 /. f -> ff;
rHd2 = norm[RicciTensor] /. f -> ff;
rHd3 = norm[rie0] /. f -> ff;

$$\in (\alpha \text{rHd1} (\text{Log}[r^2 \mu^2]) + \beta \text{rHd2} (\text{Log}[r^2 \mu^2]) + \gamma \text{rHd3} (\text{Log}[r^2 \mu^2])) // \text{Simplify};$$

ind = (%) * 4 Pi r^2 /. {f -> ff} // Simplify // sr

```

Out[23]=

$$\frac{16 \pi (-24 M q^2 r \gamma + 12 M^2 r^2 \gamma + q^4 (\beta + 14 \gamma)) \in \text{Log}[r^2 \mu^2]}{r^6}$$

```

In[24]:= int[r_] = Integrate[ind, r];
int[rt] - int[rh] // Simplify;
Limit[%, rt -> Infinity];
rInt = 1 / tem0 * % /. rh -> rh0 /. M -> mh0 // FullSimplify // sr
freehd = -tem0 * rInt // Simplify

```

Out[27]=

$$\frac{1}{75 \text{rh0}^5 \text{tem0}} 8 \pi \in (-25 q^2 \text{rh0}^2 \gamma + 100 \text{rh0}^4 \gamma + q^4 (12 \beta + 43 \gamma) + 30 (-5 q^2 \text{rh0}^2 \gamma + 5 \text{rh0}^4 \gamma + q^4 (\beta + 4 \gamma)) \text{Log}[\text{rh0}^2 \mu^2])$$

Out[28]=

$$-\frac{1}{75 \text{rh0}^5} 8 \pi \in (-25 q^2 \text{rh0}^2 \gamma + 100 \text{rh0}^4 \gamma + q^4 (12 \beta + 43 \gamma) + 30 (-5 q^2 \text{rh0}^2 \gamma + 5 \text{rh0}^4 \gamma + q^4 (\beta + 4 \gamma)) \text{Log}[\text{rh0}^2 \mu^2])$$

Above, we have used the formula  $\log \frac{\square}{\mu^2} \text{Riemann} = -\ln(r^2 \mu^2) \text{Rie-}$  mann, which is suggested in arXiv: 2104.14902 and other papers based on several reasons. Summing the two parts (coming from  $\int R - \frac{1}{4} F^2$  and  $\epsilon \int L_{hd}$  respectively) together, we get the total free energy of the perturbed black hole:

```
In[29]:= freeqtPd = freeqt0 + freehd /. M → rh0 // Simplify // sr
          化简
```

```
Out[29]=
```

$$\frac{3 q^2 + rh0^2}{4 rh0} - \frac{1}{75 rh0^5} 8 \pi \in \left( -25 q^2 rh0^2 \gamma + 100 rh0^4 \gamma + \right. \\ \left. q^4 (12 \beta + 43 \gamma) + 30 (-5 q^2 rh0^2 \gamma + 5 rh0^4 \gamma + q^4 (\beta + 4 \gamma)) \log[rh0^2 \mu^2] \right)$$

## 2. The thermodynamic quantities followed from the perturbed free energy.

### (1) The calculation of thermodynamics quantities:

The expressions for  $rh0^{(1,0)}[T, q]$ ,  $rh0^{(0,1)}[T, q]$  is given below. They are useful when taking the derivatives of the free energy with respect to T and q by the chain rule of calculus.

```
In[30]:= Outer[D, {T - (tem /. rh0 → rh0[T, q]) == 0}, {T, q}];
          外积 偏导
Solve[%[[1]], {rh0^(1,0)[T, q], rh0^(0,1)[T, q]}];
          解方程
sub = %[[1]] /. {rh0[q, T] → rh0};
```

Calculate the electrostatic potential:

```
In[33]:= phiPd =
          D[(freeqtPd /. rh0 → rh0[T, q]), q] /. sub /. rh0[T, q] → rh0 // Simplify // sr
          偏导 化简
```

```
Out[33]=
```

$$\frac{q}{rh0} + \frac{1}{75 rh0^5 (-3 q^2 + rh0^2)} \\ \in \left( 3600 \pi q rh0^4 \gamma + 16 \pi q^5 (72 \beta + 283 \gamma) + q^3 rh0^2 (-384 \pi \beta - 6176 \pi \gamma) + \right. \\ \left. 480 \pi q^3 (q^2 - 2 rh0^2) (\beta + 4 \gamma) \log[rh0^2 \mu^2] \right)$$

Calculate the entropy from the formula  $S = -dF/dT$ :

```
In[34]:= entrPd =
  -D[(freeqtPd /. rh0 -> rh0[T, q]), T] /. sub /. {rh0[T, q] -> rh0} // Simplify //
  偏导 化简
  sr
```

Out[34]=

$$\pi \text{rh}\theta^2 + \frac{1}{3 \text{rh}\theta^2 (-3 q^2 + \text{rh}\theta^2)} \pi \in (-32 \pi q^4 \gamma + 288 \pi q^2 \text{rh}\theta^2 \gamma - 256 \pi \text{rh}\theta^4 \gamma + 192 \pi (-3 q^2 \text{rh}\theta^2 \gamma + \text{rh}\theta^4 \gamma + q^4 (\beta + 4 \gamma)) \text{Log}[\text{rh}\theta^2 \mu^2])$$

Calculate the energy of the BH from the formula  $M=F+TS$ :

```
In[35]:= massPd = freeqtPd + tem * entrPd // sr
```

Out[35]=

$$\frac{q^2 + \text{rh}\theta^2}{2 \text{rh}\theta} - \frac{1}{75 \text{rh}\theta^5 (-3 q^2 + \text{rh}\theta^2)} 16 \in (-18 \pi q^6 \beta + 6 \pi q^4 \text{rh}\theta^2 \beta - 77 \pi q^6 \gamma + 184 \pi q^4 \text{rh}\theta^2 \gamma - 375 \pi q^2 \text{rh}\theta^4 \gamma + 150 \pi \text{rh}\theta^6 \gamma + 30 \pi q^6 \beta \text{Log}[\text{rh}\theta^2 \mu^2] - 60 \pi q^4 \text{rh}\theta^2 \beta \text{Log}[\text{rh}\theta^2 \mu^2] + 120 \pi q^6 \gamma \text{Log}[\text{rh}\theta^2 \mu^2] - 240 \pi q^4 \text{rh}\theta^2 \gamma \text{Log}[\text{rh}\theta^2 \mu^2])$$

## (2) The comparison with existing results in the literature:

The above results are given as the functions of  $q$  and  $\text{rh}0$ . We can also re-express them as the functions of  $q$  and  $\text{rh}$ . Note that  $\text{rh}0$  is the horizon radius of the original unperturbed BH, and  $\text{rh}$  is the horizon radius of the perturbed BH. Below, after doing so, we find that the outcome reproduces the results in arXiv: 2104.14902 that grappled with the complexities involved in deriving gravitational field equations from the nonlocal effective action and further solving the black hole metric from them.

To accomplish this, we should use the Wald entropy formula. The Wald entropy (at first order in  $\epsilon$ ) for the perturbed BH can also be obtained from the unperturbed BH solution. And it is naturally given as a function of  $r_h$ .

In[36]:= 
$$\text{entrWd} = \pi \text{rh}^2 - \epsilon \frac{32 \pi^2 \left( (\beta + 4 \gamma) q^2 - 2 \gamma \text{rh}^2 \right) \text{Log}[\text{rh}^2 \mu^2]}{\text{rh}^2} // \text{sr}$$

Out[36]=

$$\pi \text{rh}^2 - \frac{32 \pi^2 \left( -2 \text{rh}^2 \gamma + q^2 (\beta + 4 \gamma) \right) \epsilon \text{Log}[\text{rh}^2 \mu^2]}{\text{rh}^2}$$

Requiring  $\text{entr} = \text{entrWd}$ , we can derive a relation between  $\text{rh0}$  and  $\text{rh}$ .

In[37]:= 
$$\begin{aligned} & (\text{entrWd} - \text{entrPd}) /. \text{rh0} \rightarrow \text{rh} * (1 + \epsilon \text{b1}) // \text{sr}; \\ & \text{Solve}[\% == 0, \text{b1}]; \\ & \text{解方程} \\ & \text{rh0f} = \text{rh} (1 + \epsilon \text{b1}) /. \%[[1]] // \text{sr} \end{aligned}$$

Out[39]=

$$\begin{aligned} & \text{rh} + \frac{1}{3 \text{rh}^3 (-3 q^2 + \text{rh}^2)} \\ & 16 \pi \epsilon \left( q^4 \gamma - 9 q^2 \text{rh}^2 \gamma + 8 \text{rh}^4 \gamma + 3 q^4 \beta \text{Log}[\text{rh}^2 \mu^2] - 3 q^2 \text{rh}^2 \beta \text{Log}[\text{rh}^2 \mu^2] + \right. \\ & \quad \left. 12 q^4 \gamma \text{Log}[\text{rh}^2 \mu^2] - 12 q^2 \text{rh}^2 \gamma \text{Log}[\text{rh}^2 \mu^2] \right) \end{aligned}$$

Below we derive the expressions of T and M which reproduce eqs.(35) and (37) in arXiv: 2104.14902.

In[40]:= 
$$\begin{aligned} & \text{tem} /. \text{rh0} \rightarrow \text{rh0f} // \text{Simplify} // \text{sr} \\ & \text{化简} \\ & \text{massPd} /. \text{rh0} \rightarrow \text{rh0f} // \text{Simplify} // \text{sr} \\ & \text{化简} \end{aligned}$$

Out[40]=

$$\begin{aligned} & \frac{-q^2 + \text{rh}^2}{4 \pi \text{rh}^3} - \frac{1}{3 \text{rh}^7} 4 \epsilon \left( q^4 \gamma - 9 q^2 \text{rh}^2 \gamma + 8 \text{rh}^4 \gamma + 3 q^4 \beta \text{Log}[\text{rh}^2 \mu^2] - \right. \\ & \quad \left. 3 q^2 \text{rh}^2 \beta \text{Log}[\text{rh}^2 \mu^2] + 12 q^4 \gamma \text{Log}[\text{rh}^2 \mu^2] - 12 q^2 \text{rh}^2 \gamma \text{Log}[\text{rh}^2 \mu^2] \right) \end{aligned}$$

Out[41]=

$$\begin{aligned} & \frac{q^2 + \text{rh}^2}{2 \text{rh}} - \frac{1}{75 \text{rh}^5} 8 \epsilon \left( 12 \pi q^4 \beta + 43 \pi q^4 \gamma - 25 \pi q^2 \text{rh}^2 \gamma + 100 \pi \text{rh}^4 \gamma - 45 \pi q^4 \beta \text{Log}[\text{rh}^2 \mu^2] + \right. \\ & \quad \left. 75 \pi q^2 \text{rh}^2 \beta \text{Log}[\text{rh}^2 \mu^2] - 180 \pi q^4 \gamma \text{Log}[\text{rh}^2 \mu^2] + 300 \pi q^2 \text{rh}^2 \gamma \text{Log}[\text{rh}^2 \mu^2] \right) \end{aligned}$$

### 3. The test of the weak gravity conjecture.

Taking the  $T \rightarrow 0$  limit, which implies  $q \rightarrow \text{rh0}$  due to the formula

$T = -\frac{q^2}{4\pi rh_0^3} + \frac{1}{4\pi rh_0}$ . We find the expressions for the mass and entropy:

In[42]:= `massPd /. rh0 -> q // Simplify;`  
[化简]

`massPdExt = % /. {β ->  $\frac{1}{11520\pi^2}(-2ns + 8nf + 176nv + 52)$ ,`  
`γ ->  $\frac{1}{11520\pi^2}(2ns + 7nf - 26nv + 398)$ } // Simplify // sr`  
[化简]

Out[43]=

$$q + \frac{\epsilon \left( -23794 - 461nf - 106ns + 478nv - 90(274 + 6nf + ns + 12nv) \operatorname{Log}[q^2 \mu^2] \right)}{54000\pi q}$$

In[44]:= `entrPd /. rh0 -> q // Simplify;`  
[化简]

`entrPdExt = % /. {β ->  $\frac{1}{11520\pi^2}(-2ns + 8nf + 176nv + 52)$ ,`  
`γ ->  $\frac{1}{11520\pi^2}(2ns + 7nf - 26nv + 398)$ } // Simplify // sr`  
[化简]

Out[45]=

$$\pi q^2 - \frac{1}{180} (424 + 11nf + ns + 62nv) \epsilon \operatorname{Log}[q^2 \mu^2]$$

The  $\frac{dM_{\text{ext}}}{d\epsilon}$  at fixed charge  $q$  can be straightforwardly obtained as

In[46]:= `D[massPdExt, ε]`  
[偏导]

Out[46]=

$$\frac{-23794 - 461nf - 106ns + 478nv - 90(274 + 6nf + ns + 12nv) \operatorname{Log}[q^2 \mu^2]}{54000\pi q}$$

As explained in arXiv:2312.07127, the  $\frac{dM_{\text{ext}}}{d\epsilon}$  at fixed charge  $q$  can also be obtained from the  $T \rightarrow 0$  limit of  $\frac{dF}{d\epsilon}$  at fixed  $T$  and  $q$  (which means fixed  $rh_0$  and  $q$ ). Computing the expression for  $\frac{dF}{d\epsilon}$  and taking the  $T \rightarrow 0$  limit, it gives

```

In[47]:= vthEp = D[freeqtPd, ε] // FullSimplify;
          [偏导] [完全简化]
vthEp /. q → rh0 // Simplify;
          [化简]

% /. {β →  $\frac{1}{11\,520\,\pi^2} (-2\,ns + 8\,nf + 176\,nv + 52)$ ,
      γ →  $\frac{1}{11\,520\,\pi^2} (2\,ns + 7\,nf - 26\,nv + 398)$ } // Simplify
          [化简]

```

Out[49]=

$$-\frac{23\,794 + 461\,nf + 106\,ns - 478\,nv + 90\,(274 + 6\,nf + ns + 12\,nv)\,\text{Log}[\text{rh0}^2\,\mu_*^2]}{54\,000\,\pi\,\text{rh0}}$$

The subleading terms can be omitted, which are also non-universal for that they can be easily changed (or absorbed) by other local  $O(R^2)$  interactions that are model-dependent. So the universal part that we are concern about is given by

```

In[52]:= -  $\frac{1}{600\,\pi\,\text{rh0}}$  (274 + 6 nf + ns + 12 nv) Log[rh02 μ*2] // Simplify;
          [对数] [化简]

```

Here  $\mu_*$  represents some characteristic energy scale beyond which the effective field theoretical description becomes invalid, and its value might be close to Planck energy. So there is  $\text{Log}[\text{rh0}^2\,\mu_*^2] \gg 1$ .

In conclusion, **the result has a definite minus sign**, thus the weak gravity conjecture passes through the test of the one-loop effective action of quantum gravity.
